# Supplementary material for: ThinkAct: Vision-Language-Action Reasoning via Reinforced Visual Latent Planning
Source: arXiv:2507.16815 source file (2025-09-18)
Supplement: Supplementary file 1 [file contributors.tex]

\section{Contributors and Acknowledgments}
\label{sec::contributors}

\subsection{Core Contributors}
Alisson Azzolini, 
Junjie Bai,
Jiaxin Cao,
Prithvijit Chattopadhyay,
Huayu Chen, 
Yin Cui, 
Yifan Ding,
Liang Feng, 
Siddharth Gururani, 
Imad El Hanafi, 
Zekun Hao, 
Jacob Huffman, 
Jingyi Jin, 
George Kurian, 
Nayeon Lee, 
Zhaoshuo Li, 
Xuan Li, 
Maosheng Liao, 
Tsung-Yi Lin, 
Ming-Yu Liu, 
Xiangyu Lu, 
Wei Ping, 
David W. Romero,
Shuran Song, 
Lyne Tchapmi, 
Andrew Z. Wang, 
Boxin Wang, 
Haoxiang Wang, 
Fangyin Wei, 
Jiashu Xu, 
Dinghao Yang,
Xiaodong Yang, 
Zhuolin Yang, 
Jingxu Zhang, 
Xiaohui Zeng, 
Zhe Zhang

\noindent \textbf{Contributions:} 
\textbf{YC, SS, MYL, TYL} defined physical common sense and embodied reasoning ontologies. \textbf{YC, PC, JX, AZW, TYL} curated physical common sense data and benchmarks. \textbf{XY, PC, FW, XL, AZW, SG, TYL} curated embodied reasoning data and benchmark. \textbf{ZL, JJ, TYL} designed the captioning method. \textbf{JX, ZH, LT, JJ, XL, ZL, SG, TYL} curated self-supervised data and benchmark. \textbf{YC, PC, SG} post-processed extracted reasoning traces. \textbf{BW, NL, ZY, WP} trained the base VLM models. \textbf{DWR, HW, XZ} built the infrastructure for supervised fine-tuning. \textbf{XZ, GK, AA, HW, SG, ZL, DWR, FW, TYL} trained the Physical AI supervised fine-tuned models. \textbf{ZL, NL, FW, YD} evaluated the reasoning models. \textbf{JH, IH, ZZ, HW, ZH, DWR, AA, JC, LF, ML, XLu, DY, JZ, JB} built the reinforcement learning infrastructure. \textbf{ZH, JH, HC, JX, LT}  trained Physical AI reinforcement learning models.  \textbf{YC, TYL} organized paper writing. \textbf{MYL, TYL} designed the overall system.

\subsection{Contributors}
Hannah Brandon,
Jinju Chu,
Jenna Diamond,
Francesco Ferroni,
Rama Govindaraju,
Jinwei Gu,
Brendan Johnson,
Rizwan Khan,
Elena Lantz,
Yen-Chen Lin,
Alice Luo,
Andrew Mathau,
Yun Ni,
Lindsey Pavao,
Misha Smelyanskiy,
Yao Xu

\textbf{Contributions:}
\textbf{YX, LP, AM, RK, JC, BJ, EL, HB, JD} helped collect human annotations. \textbf{JG} helped with the vision encoder. \textbf{FF} curated training data. \textbf{YN, RG, MS} supported scaling model training infrastructure. \textbf{YCL} provided insights on physical common sense ontology. \textbf{AL} helped with overall data curation.

\subsection{Acknowledgments}
We'd like to thank Wenliang Dai, Guo Chen, Guilin Liu, Zhiding Yu, Mohammad Shoeybi, Andrew Tao, Bryan Catanzaro for discussion and data curation of general VLM training.
Xinshuo Weng, Boris Ivanovic for data curation of AV. Moo Jin Kim for setting up a simulation environment of object permanence data collection. Heng Wang for human annotation pipeline. Pooya Jannaty for AoT idea discussion.
