# Supplementary material for: ThinkAct: Vision-Language-Action Reasoning via Reinforced Visual Latent Planning
Source: arXiv:2507.16815 source file (2025-09-18)
Supplement: Supplementary file 2 [file prompts.tex]

\section{Prompts Used for Data Curation}
\label{sec::prompts}

\subsection{Physical Common Sense Question-Construction Prompt}

\begin{tcolorbox}[colback=nvidiagreen!3,colframe=nvidiagreen!75!white,title=\textsc{Physical Common Sense Question-Construction Prompt},left=0.5ex,right=0.5ex,top=0.5ex,bottom=0.5ex]
\fontsize{9.}{9.}\selectfont
\begin{Verbatim}[breaklines=true, breaksymbolleft={}, breaksymbolright={}]
You will be given a detailed caption describing the video. Your task is to generate 6 extremely challenging questions to evaluate the reasoning ability of a state-of-the-art model that require multi-step deep reasoning from the caption.

Try your very best to use your creativity to generate extremely challenging questions!
Here is a list of categories of questions you should generate:
1. Common sense reasoning, including but not limited to:
- Physical common sense, such as gravity, balance, stability, support, elasticity, deformation, lighting, heat, motion, acceleration, etc.
- Physical attributes that are not directly mentioned in the caption, such as mass, temperature, etc.
- Object state changes, such as egg changed from liquid to solid, steak changed from raw to cooked, etc.
- Object permanence, such as object visibility, occlusion, etc.

2. Spatial reasoning, including but not limited to:
- Spatial plausibility, such as whether the object can be placed in a certain location, in a certain orientation, etc.
- Affordance, such as whether the object can be used for a certain purpose, etc.
- Scene or surrounding environment that is not directly mentioned in the caption, such as in a tunnel, underwater, weather (sunny, rainy, etc.), etc.

3. Temporal reasoning, including but not limited to:
- Complex action understanding, such as subtask or goal decomposition, whether a task is completed, etc.
- Temporal order of events, such as before/after/simultaneously, etc.
- Planning, such as whether the object can be used for a certain purpose, come up with a plan based on the video, what are the next steps, etc.

Below are some additional rules you must follow:
1. You must create questions that require both the information in the caption and the external knowledge to challenge the model's reasoning ability with your creativity.
2. You must NOT create any questions with answers that are directly given in the caption.
3. You must NOT create any questions that can be answered by external knowledge only without the information from the video caption.
4. When asking questions, you should give as little information as possible. The model you are evaluating on is expected to get any information needed to answer the question from the video itself.

In your 6 questions, 2 of them should be about common sense reasoning and planning using world knowledge, 2 of them should be about spatial reasoning, and 2 of them should be about temporal reasoning.

You question should be concise with a maximum of 10 words.

This is the caption:
{caption}

You should treat video caption as the video. Focus on the video itself and do not mention anything related to the captions. For example, you should not mention "the caption", "the description", "what is mentioned", etc.

Instead, you can use wordings like "in the video", "the video shows", etc.
\end{Verbatim}
\label{prompt:commonsense_reasoning_question_construction}
\end{tcolorbox}

\subsection{Physical Common Sense Reasoning Extraction Prompt}

\begin{tcolorbox}[colback=nvidiagreen!3,colframe=nvidiagreen!75!white,title=\textsc{Physical Common Sense Reasoning Extraction Prompt},left=0.5ex,right=0.5ex,top=0.5ex,bottom=0.5ex]
\fontsize{9.}{9.}\selectfont
\begin{Verbatim}[breaklines=true, breaksymbolleft={}, breaksymbolright={}]
This is the video you see:
This video showcases noodles being prepared. 

The video begins with someone standing by a large boiling pot and putting noodles into one of six small circular compartments dipped into boiling water in a large circular stainless steel pot. The compartments are also stainless steel. The person using their right hand, stirs the noodles in a circular motion using light brown wooden chopsticks, and their left holds the compartment into place using a dark metallic stick-like object. The pot is placed on a black burner. Steam rises from the pot, and bubbles form, indicating active boiling. The person cooking is wearing a grey top with the sleeves reaching his elbow and has a rope tied to their waist.

The setup includes a stainless steel surface stained with white drops, a silver pot filler tap above the boiling pot, and on its left there are two deep silver filters. A stainless steel pot with a stainless steel lid on the cooking pot's left, and a white cloth placed on the lid. The background also includes a big spoon next to the burner used to cook the noodles. The lighting is bright, causing reflections and shadows over the silver surface. The camera keeps alternating a push-in and a push-out motion in a medium shot over a high angle, providing a clear, unobstructed view of the cooking process.

Answer the following question:
What would happen if the pot was not boiling?
\end{Verbatim}
\label{prompt:commonsense_reasoning_extraction}
\end{tcolorbox}

\subsection{AgiBot Reasoning Extraction Prompt}

\begin{tcolorbox}[colback=nvidiagreen!3,colframe=nvidiagreen!75!white,title=\textsc{AgiBot Reasoning Extraction Prompt},left=0.5ex,right=0.5ex,top=0.5ex,bottom=0.5ex]
\fontsize{9.}{9.}\selectfont
\begin{Verbatim}[breaklines=true, breaksymbolleft={}, breaksymbolright={}]
The state of the environment is as follows:
Inside a supermarket near a fruit stand. Well-lit indoor environment with artificial lighting. The floor appears to be tiled, and the overall ambiance suggests a clean and organized retail space. 

Camera - Positioned at a medium height, slightly above the fruit stand, capturing the robot arms and the fruit stand from a frontal perspective. The camera provides a clear, steady shot focusing on the interaction between the robot arms and the fruits. It captures the details of the objects in the foreground while keeping the background slightly out of focus. The camera remains stationary, providing a stable view of the robot arms and the fruit stand. 

Fruit Stand - Center of the frame, consisting of wooden trays filled with various fruits. The fruit stand has multiple compartments made of light-colored wood. It contains a variety of fruits such as bananas, oranges, apples, pears, and others, arranged neatly in rows. 

Shopping Cart - In the foreground, partially visible under the robot arms. A standard metal shopping cart with red handles and a basket containing some items, including a plastic bag where the apple is being placed. 

Plastic Bag - Hanging from the shopping cart, below the robot arms. A transparent plastic bag with some red items inside, likely other fruits or vegetables. Hanging from the shopping cart, partially filled with items. Receives the red apple dropped by Robot Arm 2. 

Grapes - Held by Robot Arm 1, positioned over the fruit stand. A cluster of dark purple grapes, appearing fresh and ripe. 

Apple - Held by Robot Arm 2, positioned over the plastic bag in the shopping cart. A single red apple, shiny and smooth, indicating freshness.

A robot is performing the following task (may not be finished in the video): Pickup items in the supermarket

This is how the robot's actions impact the environment:

Robot Arm 1 - On the left side of the frame, extending towards the fruit stand. A mechanical arm with a black and white color scheme. It has a gripper mechanism at the end holding a bunch of grapes. The arm is articulated with joints allowing for precise movement. Holds a bunch of grapes with its grippers, positioned over the fruit stand.

Robot Arm 2 - On the right side of the frame, extending towards the fruit stand. Another mechanical arm similar in design to Robot Arm 1 but with a different configuration of the gripper mechanism. It is holding an apple and appears to be placing it into a plastic bag. Holds a red apple with its grippers, positioned above the plastic bag in the shopping cart. Releases the red apple into the plastic bag in the shopping cart.


**Output Requirements**:
- Predict the next immediate action of the robot.

**Response Format**:
- <action> your predicted action </action>.
\end{Verbatim}
\label{prompt:agibot_reasoning}
\end{tcolorbox}

\subsection{Spatial Puzzle Reasoning Extraction Prompt}

\begin{tcolorbox}[colback=nvidiagreen!3,colframe=nvidiagreen!75!white,title=\textsc{Spatial Puzzle Reasoning Extraction Prompt},left=0.5ex,right=0.5ex,top=0.5ex,bottom=0.5ex]
\fontsize{9.}{9.}\selectfont
\begin{Verbatim}[breaklines=true, breaksymbolleft={}, breaksymbolright={}]
You will be given a puzzle, which has 8 images, each broken into a 2x2 grid: top-left, top-right, bottom-left, bottom-right.
As a result, there are 32 frames and the first frame shows that "{first_frame_caption}".

{frames_and_captions}

For the remaining 31 frames, which three are most likely to be from the same images as the first frame? Then among the three, which one is most likely to be at {direction} of the first frame?

Give your answer in the following format:
<answer>
Same image: Frame a, Frame b, Frame c
{direction}: Frame d
</answer>
\end{Verbatim}
\label{prompt:puzzle_reasoning_prompt}
\end{tcolorbox}

\subsection{Arrow of Time Reasoning Extraction Prompt}

\begin{tcolorbox}[colback=nvidiagreen!3,colframe=nvidiagreen!75!white,title=\textsc{Arrow of Time Reasoning Extraction Prompt for forward video, backward video prompt is similar},left=0.5ex,right=0.5ex,top=0.5ex,bottom=0.5ex]
\fontsize{9.}{9.}\selectfont
\textbf{\underline{HUMAN TURN:}}
\begin{Verbatim}[breaklines=true, breaksymbolleft={}, breaksymbolright={}]
Here is a sequence of frames. Is it playing forward or backward?
\end{Verbatim}

\noindent\hdashrule{\linewidth}{0.4pt}{2pt}

\textbf{\underline{ASSISTANT TURN:}}
\begin{Verbatim}[breaklines=true, breaksymbolleft={}, breaksymbolright={}]
The video is playing forward.
\end{Verbatim}
\noindent\hdashrule{\linewidth}{0.4pt}{2pt}
\textbf{\underline{HUMAN TURN:}}
\begin{Verbatim}[breaklines=true, breaksymbolleft={}, breaksymbolright={}]
So here is a forward-playing video. Describe in details what visual clues do you notice that indicate the time is going forward i.e. the video is not reversed? Please avoid repeating the question and refrain from using bullet points. Present the evidence but no need to give the verdict.
\end{Verbatim}
\label{prompt:aot_reasoning_prompt}
\end{tcolorbox}

\subsection{Object Permanence Reasoning Extraction Prompt}

\begin{tcolorbox}[colback=nvidiagreen!3,colframe=nvidiagreen!75!white,title=\textsc{Object Permanence Reasoning Extraction Prompt},left=0.5ex,right=0.5ex,top=0.5ex,bottom=0.5ex]
\fontsize{9.}{9.}\selectfont
\begin{Verbatim}[breaklines=true, breaksymbolleft={}, breaksymbolright={}]
This is a video of a robotic simulation environment. The robotic arm moves and may occlude objects. The camera moves around the scene and then returns to a position near its initial location. Occlusion can also occur due to the camera's movement.

The objects in the videos are akita black bowl and akita black bowl and cookies and glazed rim porcelain ramekin and plate and wooden cabinet and flat stove.

akita black bowl is occluded in the middle of video and then vanishes unexpectedly.

Is there an object that becomes temporarily occluded but does not reappear in the end, contradicting object permanence?

Please answer the question in the following format: <think> your reasoning </think> <answer> your answer </answer>.
\end{Verbatim}
\label{prompt:permanence_reasoning_prompt}
\end{tcolorbox}
