# Supplementary material for: ThinkAct: Vision-Language-Action Reasoning via Reinforced Visual Latent Planning
Source: arXiv:2507.16815 source file (2025-09-18)
Supplement: Supplementary file 3 [file additional_results.tex]

\newpage
\section{Additional results}
\label{sec::additional_results}

\input{figures/6_experiment/fig_puzzle_example}
\input{figures/6_experiment/fig_object_example}
